# Supplementary material for: Outlier-Robust Spatial Perception: Hardness, General-Purpose Algorithms, and Guarantees
Source: arXiv:1903.11683 source file (2019-07-29)
Supplement: Supplementary file 2 [file arXiv_supp_SLAM.tex]

%!TEX root = supplemental.tex

\newpage
\clearpage
\subsection{Supplemental for Robust SLAM}
\label{sec:supp_slam}

\input{supp_fig-slam}
