# Supplementary material for: Outlier-Robust Spatial Perception: Hardness, General-Purpose Algorithms, and Guarantees
Source: arXiv:1903.11683 source file (2019-07-29)
Supplement: Supplementary file 3 [file supp_guarantees.tex]

\section{Proof of Theorem~\ref{th:guarantees}}
\label{sec:supp_guarantees}

First observe that $\res^\star_{|\selSet|}\leq \res(\selSet)$.  This holds true due to the definition of $\res^\star_{|\selSet|}$ as the smallest value of $\res(\cdot)$ among all sets with cardinality $|\selSet|$. Next, define the quantities:
\begin{itemize}
	\item $f(\selSet)\doteq \res(\emptyset)-\res(\selSet)$;
	\item $f^\star\doteq \res(\emptyset)-\res^\star_{|\selSet|}$.
\end{itemize}
We observe that:
\begin{align*}
f^\star&= \res(\emptyset)-\res^\star_{|\selSet|}\\
&\leq \res(\emptyset)\\
&= \res(\emptyset)+\res(\selSet)-\res(\selSet)\\
&=f(\selSet)+\res(\selSet).
\end{align*}
The above now imples:
\begin{align*}
\frac{f(\selSet)}{f^\star}&\geq 1- \frac{\res(\selSet)}{f^\star} \\
&\geq 1- \frac{\res(\selSet)}{f(\selSet)},
\end{align*}
where the latter holds since $f(\selSet)\leq f^\star$, which in turns holds because $\res(\selSet)\geq \res^\star$.  Finally, the above is:
\begin{align*}
\frac{f(\selSet)}{f^\star}&\geq 1- \apost_\selSet,
\end{align*}
which gives:
\begin{align*}
\res(\emptyset)-\res(\selSet)&\geq (1- \apost_\selSet)\res(\emptyset)- (1- \apost_\selSet)\res^\star_{|\selSet|} \Rightarrow\\
\apost_\selSet(\res(\emptyset)-\res^\star_{|\selSet|})&\geq \res(\selSet)-\res^\star_{|\selSet|}
\end{align*}
which gives eq.~\eqref{eq:guarantees}.  

To prove eq.~\eqref{eq:bound_refined}, we first observe that $\res^\star\geq \res^\star_{|\selSet|}$, since $|\selSet| \geq |\selSet^\star|$.  Now, it can be verified that:
\begin{equation}\label{app:eq:aux_guarantees}
\frac{\res(\selSet)-\res^\star}{\res(\emptyset)-\res^\star}\leq \frac{\res(\selSet)-\res^\star_{|\selSet|}}{\res(\emptyset)-\res^\star_{|\selSet|}},
\end{equation}
since it also is $\res(\emptyset)\geq \res(\selSet)$.
Substituting eq.~\eqref{app:eq:aux_guarantees} in eq.~\eqref{eq:guarantees}, the proof of the theorem is now complete.
